# Supplementary material for: Lasercooled radium monofluoride: A molecular all-in-one probe for new physics
Source: arXiv:1302.5682 ancillary file (2020-05-22)
Supplement: Supplementary file 1 [file Suppl.pdf]

# Supplementary material to the article “Lasercooled radium monofluoride: A molecular all-in-one probe for new physics”

Timur Isaev and Robert Berger

November 21, 2013

## FS RCC-SD calculations of the low-lying RaF electronic states

### Basis sets and nuclear model

1. The nuclear density is modelled by a spherical Gaussian distribution $\rho(R) = \rho_0 \mathrm{e}^{-\frac{3R^2}{2\xi}}$, where $\rho_0$ is the normalisation constant ( $\rho_0 = (\frac{3}{2\pi\xi})^{3/2} Z$, $Z$ is the nucleus charge in atomic units), $\xi$ is the root mean square radius of the corresponding nucleus computed according to the empirical formula $\xi/\mathrm{fm} = 0.836 A^{1/3} + 0.57$, where $A$ is the given isotope mass number. Exponent coefficients are given in $a_0^{-2}$ units. DIRAC output:

```
-----------------
  Nuclear Gaussian exponent for atom of charge  88.000 :    1.3101367628D+08
  Nuclear Gaussian exponent for atom of charge   9.000 :    5.3546911034D+08
-----------------
```

```
2.Exponents of atomic RCC-ANO basis set from EMSL library on Ra
  s                           p                    d                  f
 54615913.6000000015    22902995.8999999985  12219.0530000000   787.3961570000
 13644310.5999999996     4560028.1699999999   5143.3747900000   365.0466460000
 4219580.9900000002      1106448.3100000001   2222.3780400000   175.4953600000
 1412175.8500000001      304836.7850000000     988.0704860000    85.1582236000
 504524.4240000000        92710.0666000000     449.7383690000    43.0008059000
 188914.8130000000        30701.9828000000     212.7046920000    21.6234842000
  73701.6788000000        11019.2921000000     103.8939650000    10.7837034000
  29665.5588000000        4275.1644700000       52.1655431000     5.3421144200
  12219.0530000000         1780.8158300000      26.4523340000     2.4713129300
   5143.3747900000          787.3961570000      13.2328053000     0.9885251700
   2222.3780400000          365.0466460000       6.6044317000     0.3213940000
    988.0704860000          175.4953600000       3.0981751600     0.1285578000
    449.7383690000           85.1582236000       1.4305005600
    212.7046920000           43.0008059000       0.5970985000
    103.8939650000           21.6234842000       0.2410460000
```

```
     52.1655431000          10.7837034000        0.0973090000
     26.4523340000           5.3421144200        0.0392830000
     13.2328053000           2.4713129300
      6.6044317000           1.1390980800
      3.0981751600           0.4183576900
      1.4305005600           0.1563284900
      0.5970985000           0.0625314000
      0.2539563900           0.0250125600
      0.1015825600           0.0100050200
      0.0406330200           0.0040020100
      0.0162532100
      0.0065012800
      0.0026005100
```

```
Exponents of atomic basis set on F
  s                p          d
 103109.46      245.33029   5.0000000
 15281.007      56.919005   1.7500000
 3441.5392      17.604568   .61250000
 967.09483      6.2749950   .21437500
 314.03534      2.4470300
 113.44230      .99506000
 44.644727      .40397300
 18.942874      .15481000
 8.5327430      .05418400
 3.9194010
 1.5681570
 .62329000
 .24086100
 .08430100
```

**Influence of g-functions on Ra basis on transition energies**

```
DIRAC12 input:
---------------------
**DIRAC
.TITLE
 RCC-FS RaF calculations
.WAVE F
**HAMILTONIAN
.LVCORR
**WAVE FUNCTION
.DHF
.RELCCSD
*DHFCAL
.CLOSED SHELL
96
.MAXITR
 50
**MOLTRA
```

```
.ACTIVE
energy -2.  1000.  0.1
**END OF

 &RELCCSD DOFSPC=T DOENER=F &END
 &CCFSPC MAXIT=50, NACTP=6,6 FSSECT=1,1,0,0,0,0      &END
---------------------
Internuclear distance is 4.3 a_0.

Results with basis sets given above:
Ra00        1      88     325     325      L  - [28s25p17d12f|28s25p17d12f]
                          609     609      S  - [25s28p25d17f12g|25s28p25d17f12g]
F00         1       9      65      65      L  - [14s9p4d|14s9p4d]
                          145     145      S  - [9s14p9d4f|9s14p9d4f]

    1        0.000000000          0.000000     1|   1|   0|   0|   0|   0|   0|   0|
    2        1.644454972      13263.425194     1|   1|   0|   0|   0|   0|   0|   0|
    3        1.862216082      15019.787171     0|   0|   1|   1|   0|   0|   0|   0|
    4        1.910029611      15405.429336     0|   0|   1|   1|   0|   0|   0|   0|
    5        1.963891944      15839.858394     0|   0|   0|   0|   1|   1|   0|   0|
    6        2.068256579      16681.616029     1|   1|   0|   0|   0|   0|   0|   0|

Results with basis sets given above + 3 G-functions added from ECP Ra basis
with the exponents   0.59710; 0.25396; 0.10987:
 Ra00        1      88     370     370      L  - [28s25p17d12f3g|28s25p17d12f3g]
                           672     672      S  - [25s28p25d17f12g3h|25s28p25d17f12g3h]
 F00         1       9      65      65      L  - [14s9p4d|14s9p4d]
                           145     145      S  - [9s14p9d4f|9s14p9d4f]

    1        0.000000000          0.000000     1|   1|   0|   0|   0|   0|   0|   0|
    2        1.634267610      13181.258567     1|   1|   0|   0|   0|   0|   0|   0|
    3        1.806025286      14566.577796     0|   0|   1|   1|   0|   0|   0|   0|
    4        1.895826075      15290.870077     0|   0|   1|   1|   0|   0|   0|   0|
    5        1.908161185      15390.359462     0|   0|   0|   0|   1|   1|   0|   0|
    6        2.059582847      16611.657651     1|   1|   0|   0|   0|   0|   0|   0|
```

### Raw data for the RaF low-lying states

```
Raw data on FS-CCSD energy (in Mathematica format) at different internuclear distances
All energies are shifted by -25130.0 E_h.
Ground \Sigma_1/2 state:
{{3.4, -2.61896827} , {3.7, -2.6810475693}, {3.9, -2.701438115},
{4.0, -2.707355929}, {4.1, -2.71107952}, {4.15, -2.712245222046},
{4.2, -2.7130062}, {4.25, -2.7134023758}, {4.3, -2.7134702786},
{4.4, -2.71275215884}, {4.5, -2.711086221825} , {4.7, -2.7056587},
{5.0, -2.694317976377}, {5.5, -2.672360131139}}
First excited (\Pi_1/2):
{{3.4, -2.55914478}, {3.7, -2.620627218741}, {3.9, -2.64091361},
{4.0, -2.646828821}, {4.1, -2.650570973}, {4.15, -2.651751778991},
```

```
{4.2, -2.65253083}, {4.25, -2.65294745}, {4.3,-2.653037666863},
{4.4, -2.6523680724}, {4.5, -2.650753595208}, {4.7, -2.6454302},
{5.0, -2.634233283523}, {5.5, -2.612462214729}}
2nd excited (\Pi_3/2+\Delta_3/2):
{{3.4, -2.551178387668}, {3.7, -2.61206742}, {3.9, -2.63216039},
{4.0, -2.63814297}, {4.1, -2.64206593}, {4.15, -2.643361819482},
{4.2, -2.64426494}, {4.25, -2.64481137}, {4.3, -2.64503509},
{4.4, -2.64463889}, {4.5, -2.643301941935}, {4.7, -2.6385357},
{5.0, -2.628161427147}, {5.5, -2.607683096769}}
3rd excited (\Pi_3/2+\Delta_3/2):
{{3.4, -2.547995013745}, {3.7, -2.61050150}, {3.9, -2.63125097},
{4.0, -2.63724423}, {4.1, -2.64096208}, {4.15, -2.642110746598},
{4.2, -2.64285196}, {4.25, -2.64322834}, {4.3, -2.64327798},
{4.4, -2.64253077}, {4.5, -2.640847235558}, {4.7, -2.635417596957},
{5.0, -2.624139970427}, {5.5, -2.602951138640}}
4th excited (\Delta_5/2):
{{3.4, -2.545390225903}, {3.7, -2.60766727}, {3.9, -2.62839117},
{4.0, -2.63450950}, {4.1, -2.63844850}, {4.15, -2.639726110290},
{4.2, -2.64060121}, {4.25, -2.64111330}, {4.3, -2.64129857},
{4.4,-2.64081834}, {4.5, -2.639392742032}, {4.7, -2.634446697961},
{5.0, -2.623813022317}, {5.5, -2.602403068209}}
5th excited (\Sigma_1/2 state):
{{3.4, -2.538839380264}, {3.7, -2.60209643}, {3.9, -2.62351221},
{4.0, -2.62994016}, {4.1, -2.63415707}, {4.15, -2.635561158826},
{4.2, -2.63655436}, {4.25, -2.63717627}, {4.3, -2.63746324},
{4.4, -2.63716298}, {4.5, -2.635888067583}, {4.7, -2.631166233721},
{5.0, -2.620716634014}, {5.5, -2.599905982435}}
```

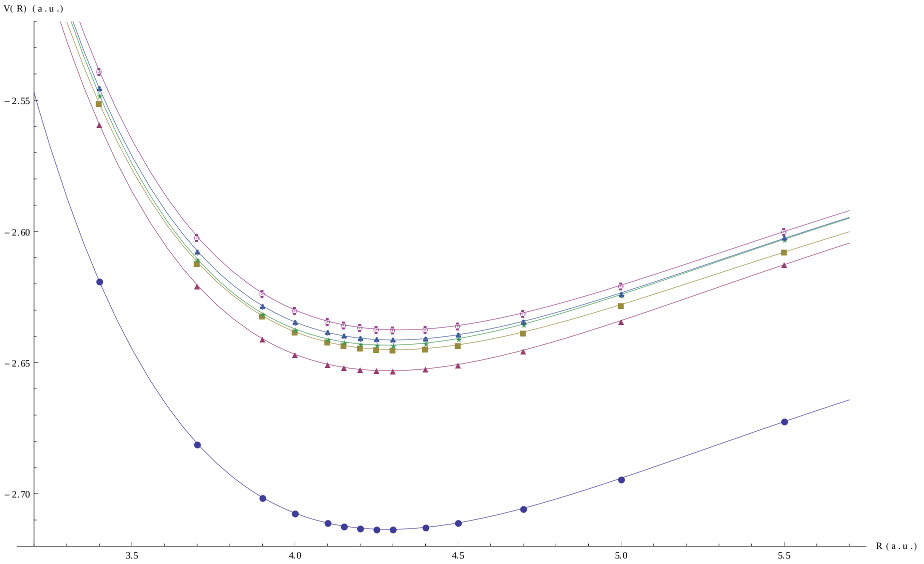


Figure 1: Fitting of the six lowest-lying electronic states by Morse potential

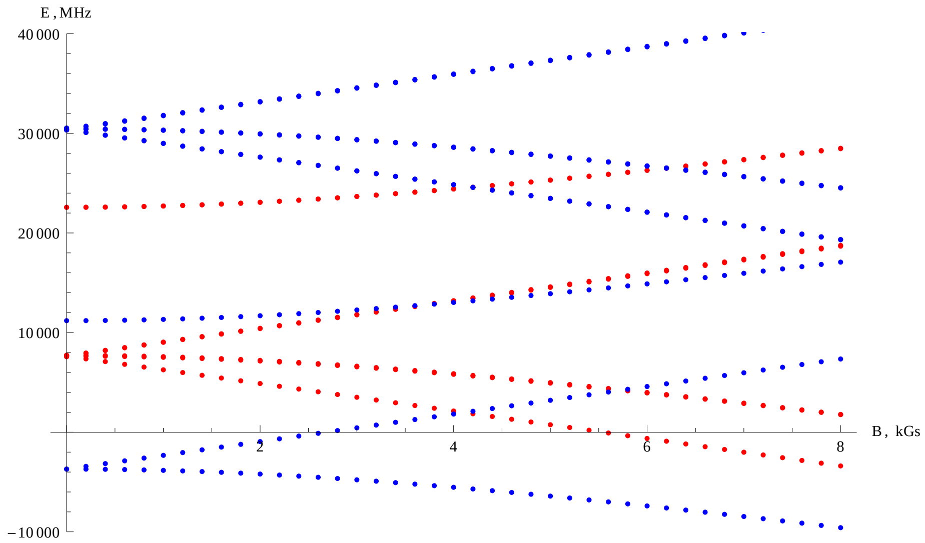


Figure 2: Level crossing in magnetic field for the spin-rotational terms of the ground electronic state of $^{225}$RaF with the projection of the total angular momentum M=−1/2 on the direction of the magnetic field. Levels of negative parity are blue and of positive parity are red.

# Crossings of the levels in magnetic field.

Spin-rotational hamiltonian is the one taken from M.G. Kozlov, L.N. Labzowskii, and A.O. Mitruschenkov "Parity nonconservation in diatomics in strong magnetic field" JETP, 73, 415 (1991). In spin-rotational hamiltonian the following parameters are used:

```
B = 5689 MHz
\delta = -2 B + 334 MHz (Estimated from DHF calculations in DIRAC)
Apar_Ra =  -15100 MHz   (ZORA calculations with modified TURBOMOLE package [1])
Aperp_Ra = -14800 MHz   (ZORA calculations with modified TURBOMOLE package [1])
Apar_F = 0
Aperp_F = 0
Gpar = 1.993   (Taken from HgF, but its variation does not much change results)
Gperp = 1.961  (Taken from HgF, but its variation does not much change results)
```

REFERENCE:

[1]. R. Alrichs, M. Bär, M. Häser, H. Horn and C. Kölmel, Chem. Phys. Lett. **162**, 165 (1989).

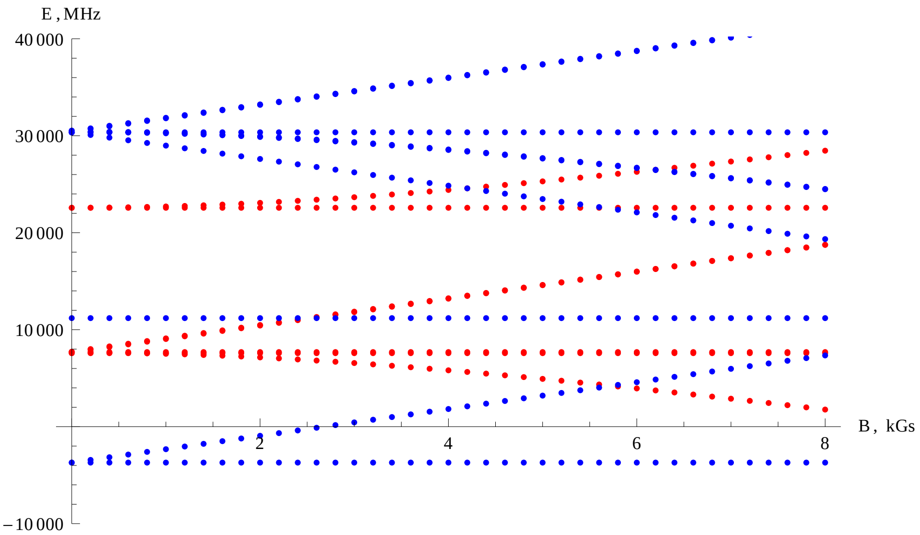


Figure 3: Level crossing in magnetic field for the spin-rotational terms of the ground electronic state of $^{225}$RaF with the projection of the total angular momentum M=−3/2 on the direction of the magnetic field. Levels of negative parity are blue and of positive parity are red.
